# Supplementary material for: Shape and Content: Incorporating Domain Knowledge into Shape Analysis
Source: arXiv:1312.6624 source file (2014-07-09)
Supplement: Supplementary file 1 [file appendix-VFS.tex]

\subsection{The Virtual File System: \DomainContent~Invariants in $\L$}
The Virtual File System (VFS)
\footnote{We present here a simplified description. The terminology
used here is different from the one used in the Linux kernel.
E.g., files are called {\em inodes} and file systems are called {\em superblocks} in the terminology of VFS.}
is comprised of various types of objects, arranged in a large number
of lists. A \emph{directory entry} (\emph{dentry) }corresponds to
a path in the file system. Both files and directories have dentries
and the dentries are arranged in a tree which is implemented by lists.
Each leaf in the dentry tree points to a \emph{file}. 
The files are partitioned between
lists depending on whether they are used or not.
A file may have more than one dentry pointing to it,
corresponding to different names of the same file.
%Each file has a list of dentries which point to it.
Other elements of the VFS which we do not
discuss further here include
\emph{file system types} and \emph{files pointers}, which are interrelated
with the above mentioned elements and stored in various lists and
other data structures.

\setlength{\intextsep}{0pt}%
\setlength{\columnsep}{0pt}%
\begin{wrapfigure}[15]{r}{31mm}
\begin{center}
\includegraphics[scale=0.85]{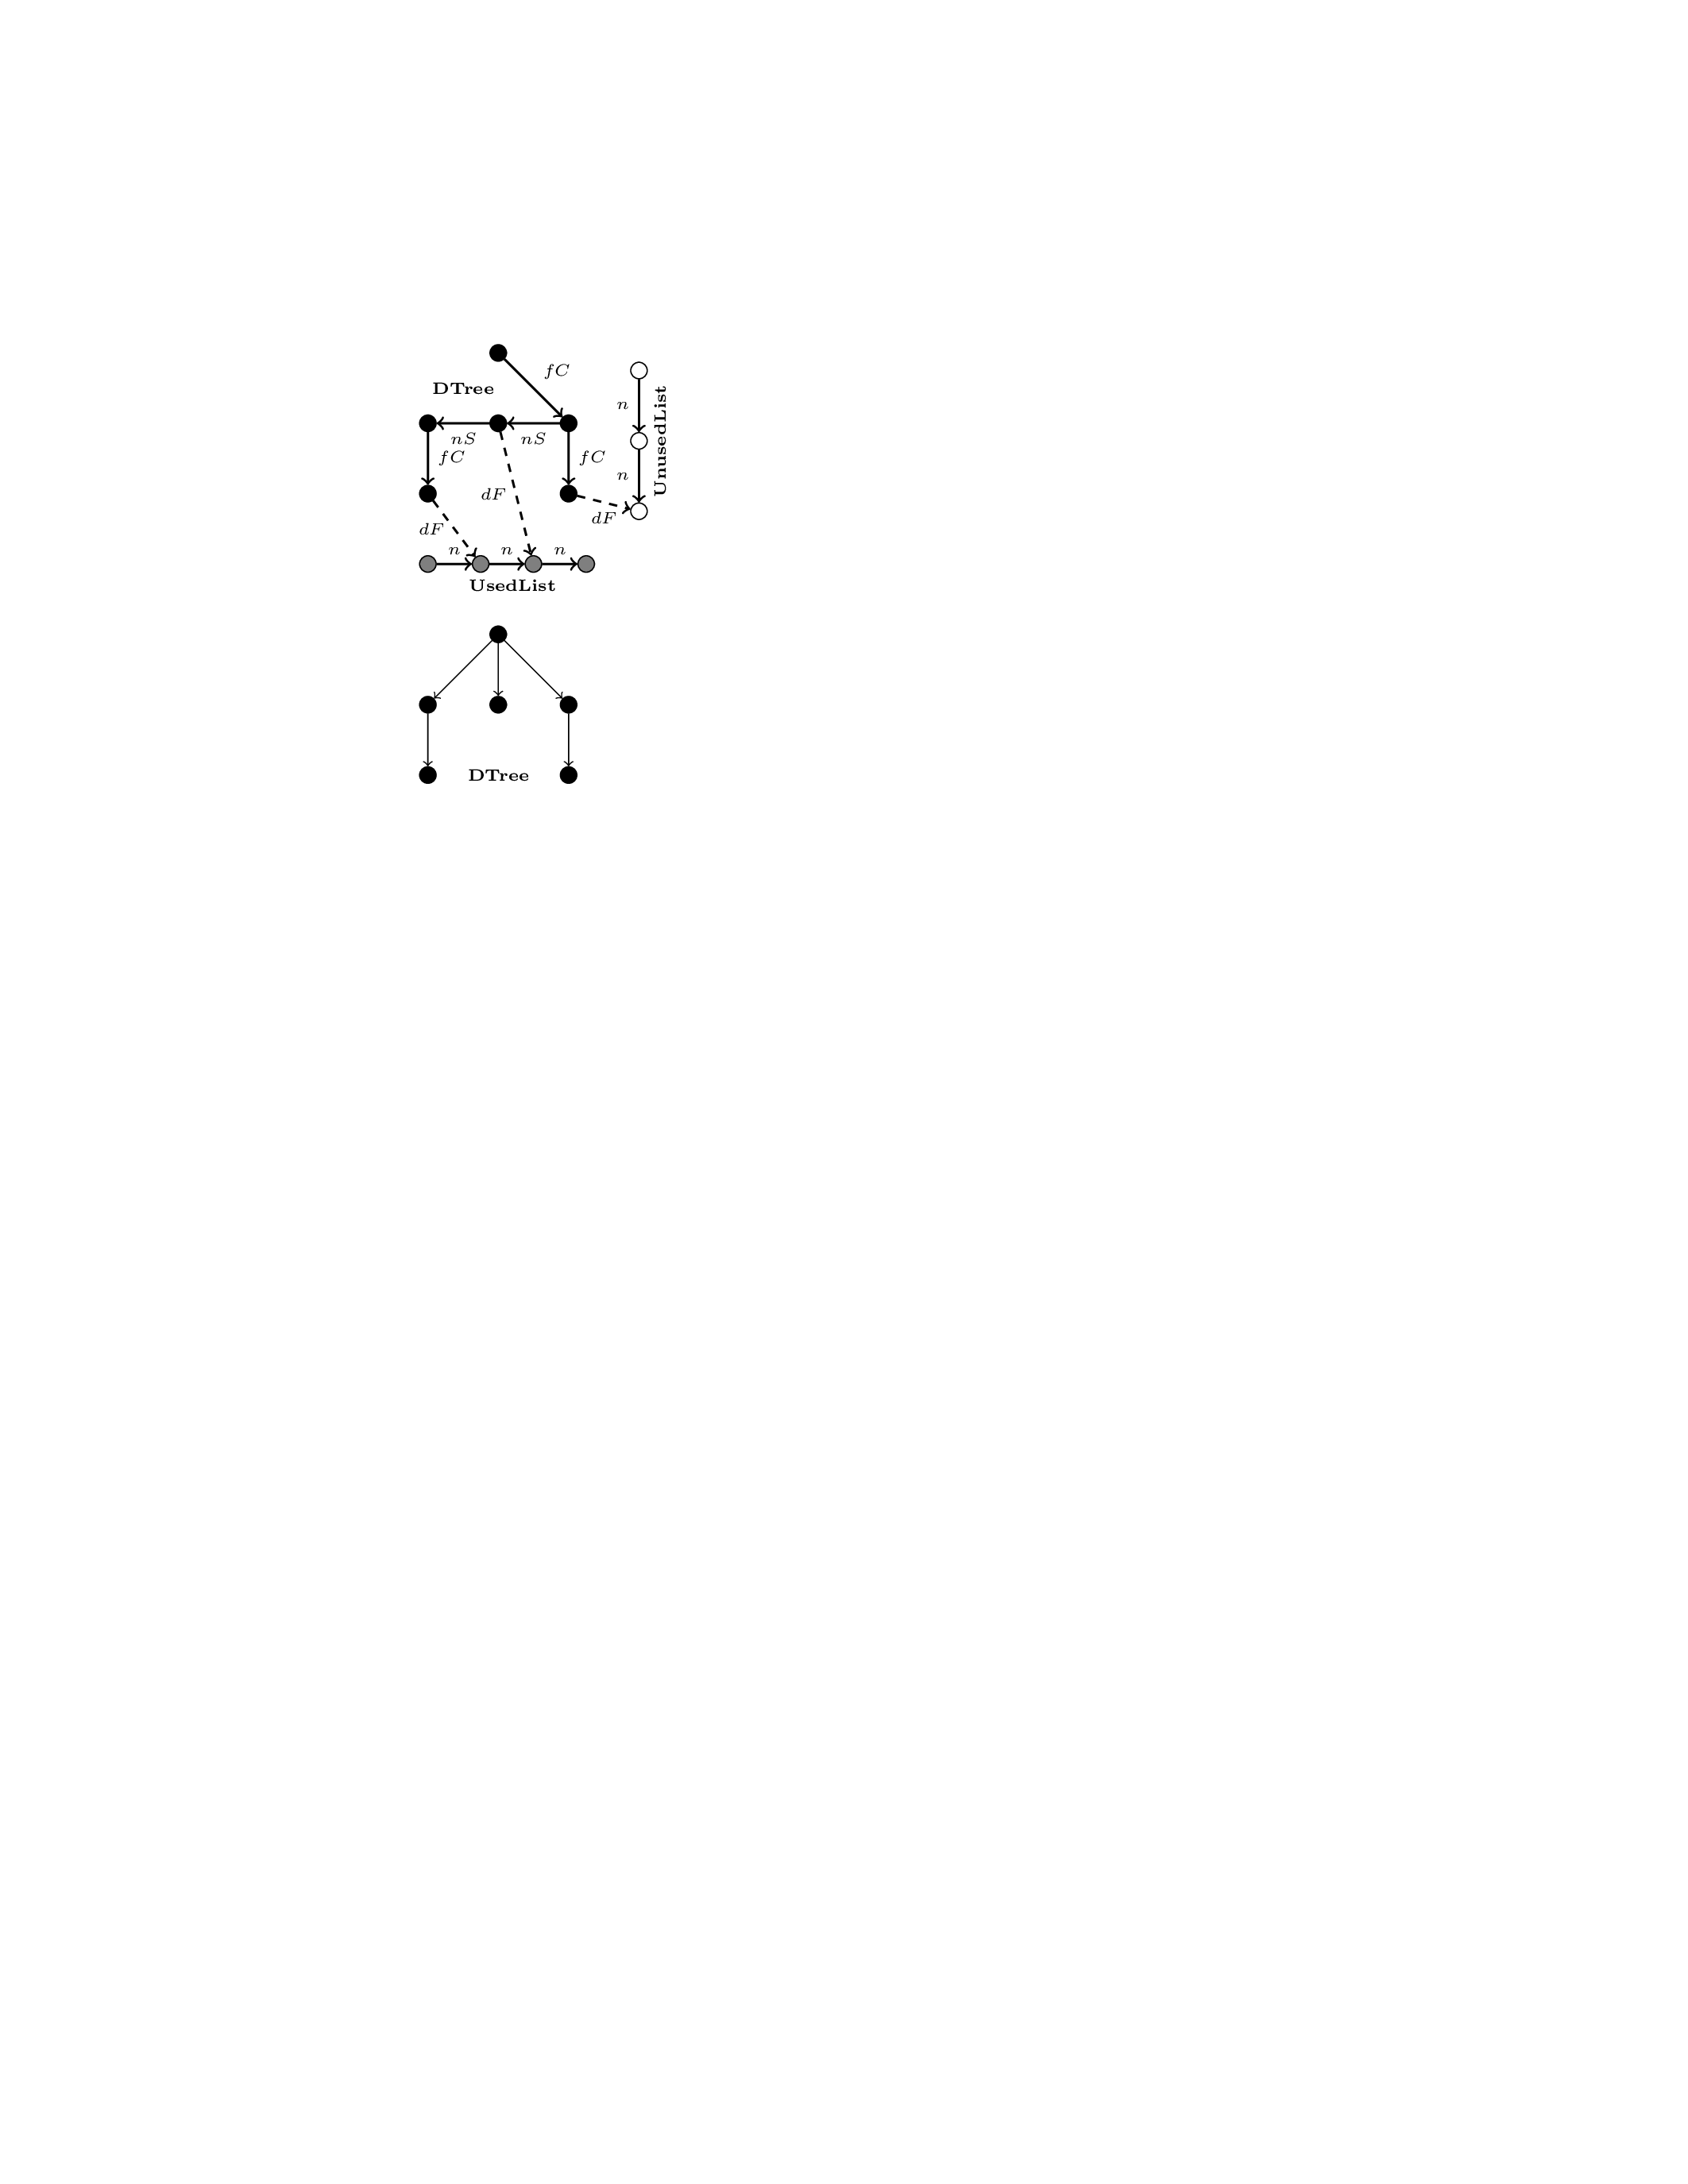}
\caption{\label{fig:VFS}}
\end{center}
\end{wrapfigure}
The concepts containing the elements of the lists and tree are respectively
$UsedList$, $UnusedList$, and $DTree$. $dentryFile$ ($dentryF$ for short) is a role corresponding to
the field pointing from dentries to files. $FileId$ is a role corresponding to a field which is considered to be the Id of the file.
The tree $DTree$ is implemented as a binary tree with three roles for the fields $firstChild$, $nextSibling$ and $parent$.
Fig. \ref{fig:VFS} illustrates the VFS. $DTree$ is represented in the memory as a binary tree with fields $fC=firstChild$ and $nS=nextSibling$ (above).
We think of it as a tree with unbounded degree (below). $n$ is short for $next$. Additionally every file in the two lists has a $FileId$ field.
The invariants of system:

\begin{enumerate}
\item The allocated memory contains three disjoint sets
of elements: $UsedList$, $UnusedList$ and $DTree$:\\
$
\begin{array}{lllllllll}
 UsedList\sqcup UnusedList\sqcup DTree & \sqsubseteq & Alloc \\
 UnusedList\sqcap DTree & \equiv & \bot\\
 UsedList\sqcap DTree & \equiv & \bot \\
 UsedList\sqcap UnusedList & \equiv & \bot
\end{array}
$
\item Null fields:\\
$
\begin{array}{clclcl}
UsedList\sqcup UnusedList & \sqsubseteq & \exists dentryF.o_{\nil} \\
DTree & \sqsubseteq & \exists FileId.o_{\nil}
\end{array}
$
\item The root of $DTree$ is a directory:\\
$
\begin{array}{llcl}
DTree \sqcap \neg \exists firstChild^-.DTree \sqcap\\
 \neg nextSibling^-.DTree
% & DTree\sqcap\exists parent.o_{\nil}
 \sqsubseteq \exists dentryF.o_{\nil}\end{array}
$
\item A file belongs to the $UsedList$ if and only if a dentry in $DTree$
points to it:\\
$
\begin{array}{clcl}
 & \exists dentryF^{-}.DTree & \equiv & UsedList\\
\end{array}
$

\item
If a dentry in $DTree$ points to a file with the pointer $dentryFile$, then
it has no children in $DTree$ (otherwise it would necessarily be a directory):
$
\begin{array}{clcl}
 & DTree \sqcap \exists dentryF.\neg o_\nil & \sqsubseteq & \exists \neg firstChild\\
\end{array}
$
\item The $FileId$ is unique with respect to the lists $UsedList$ and $UnusedFiles$:\\
$
\begin{array}{clcl}
   & func(FileId^{-} \cap \top \times (UsedList \sqcup UnusedList))
\end{array}
$

\end{enumerate}
